# Supplementary material for: Tweezers: A Framework for Security Event Detection via Event Attribution-centric Tweet Embedding
Source: arXiv:2409.08221 source file (2024-09-12)
Supplement: Supplementary file 1 [file additional_criteria.tex]

\begin{table*}[h]
\diffnote{RC1}
\ra{1.5}
\begin{mdframed}[backgroundcolor=brown!10]
\caption{Detailed Criteria for Annotating Tweets}
\adjustbox{width=.8\textwidth, center}{
\begin{tabular}{ll}
\toprule
\textbf{Type} & \textbf{Annotation Guidelines} \\ 
\midrule
\textbf{General Analysis} & Tweets are analyzed and classified based on the contained cybersecurity content. \\
\textbf{Uninformative}  & Tweets lacking clarity or detailed information for classification are marked Uninformative. \\
\textbf{Security-Related Hiring} & Tweets regarding job postings in security fields are annotated as Non-security. \\
\textbf{CVE Mentions} & Classified by detailed explanation present, otherwise annotated under Vulnerability. \\
\textbf{Mentions of Hacking Groups} & Classified based on known activities of the group; otherwise, marked Uninformative. \\
\textbf{Fraud Types} & Election fraud is annotated as non-security; other frauds as Fraud/Phishing. \\
\textbf{Security Keyword Enumeration} & Tweets listing security keywords without context are considered Uninformative. \\
\textbf{Fundraising for Security Firms} & Tweets about fundraising activities for security firms are annotated as Non-security. \\
\bottomrule
\end{tabular}}
\label{tab:additional_criteria}
\end{mdframed}
\end{table*}
